# Supplementary material for: Accurate and Robust Localization Techniques for Wireless Sensor Networks
Source: arXiv:1806.05765 source file (2018-06-14)
Supplement: Supplementary file 1 [file appendixA.tex]

\chapter{Appendix}
\label{app:publ}
