# Supplementary material for: Accurate and Robust Localization Techniques for Wireless Sensor Networks
Source: arXiv:1806.05765 source file (2018-06-14)
Supplement: Supplementary file 2 [file appendix.tex]

\chapter{}
\label{Graphical User Interface}
